# Supplementary material for: Optimal scenario design for climate emulation
Source: arXiv:2606.19302 source file (2026-09-29)
Supplement: Supplementary file 1 [file supplementary.tex]

\documentclass[11pt]{article}
\usepackage[margin=1.9cm]{geometry}
\usepackage[utf8]{inputenc}
\usepackage[backref=page]{hyperref}
\usepackage[round]{natbib}
\usepackage{tikz}
\usepackage{amsmath,amsthm,amssymb,nicefrac}
\usepackage{csquotes, booktabs, url, float, tabularx, multirow, tcolorbox}
\usepackage{algorithm, algpseudocode}
\usepackage[dvipsnames]{xcolor}
\input{maths.tex}
\usepackage{caption}
\setlength{\abovecaptionskip}{4pt plus 1pt minus 1pt}
\setlength{\belowcaptionskip}{0pt}

\usepackage{glossaries}
\usepackage{authblk}

\glsdisablehyper

\newacronym{ad}{AD}{Automatic Differentiation}
\newacronym{bc}{BC}{Black Carbon}
\newacronym{cmip}{CMIP}{Coupled Model Intercomparison Project}
\newacronym{cmip6}{CMIP6}{the sixth phase of the Coupled Model Intercomparison Project}
\newacronym{cmip7}{CMIP7}{the seventh phase of the Coupled Model Intercomparison Project}
\newacronym{cs3}{CS3}{MIT Center for Sustainability Science and Strategy}
\newacronym{damip}{DAMIP}{Detection and Attribution MIP}
\newacronym{ema}{EMA}{Exponential Moving Average}
\newacronym{emic}{EMIC}{Earth system Model of Intermediate Complexity}
\newacronym{esm}{ESM}{Earth System Model}
\newacronym{fair}{FaIR}{Finite amplitude Impulse Response}
\newacronym{geomip}{GeoMIP}{Geoengineering MIP}
\newacronym{gmst}{GMST}{Global Mean Surface Temperature}
\newacronym{ic}{IC}{Initial Condition}
\newacronym{ipcc}{IPCC}{Intergovernmental Panel on Climate Change}
\newacronym{ml}{ML}{Machine Learning}
\newacronym{mlp}{MLP}{Multi-Layer Perceptron}
\newacronym{mesm}{MESM}{MIT Earth System Model}
\newacronym{mse}{MSE}{Mean Squared Error}
\newacronym{nrmse}{NRMSE}{Normalized Root Mean Square Error}
\newacronym{scm}{SCM}{Simple Climate Model}
\newacronym{sgd}{SGD}{Stochastic Gradient Descent}

% Layout penalties
\clubpenalties 3 10000 10000 0
\widowpenalties 3 10000 10000 0
\displaywidowpenalty=10000
\relpenalty=10000
\binoppenalty=10000

%%% Commenting commands - add your own

\title{Supporting information for \\
\textbf{Optimal scenario design for climate emulation}}

\author[a,b]{Christopher B. Womack}
\author[c]{Shahine Bouabid}
\author[b]{Andrei Sokolov}
\author[b]{Popat Salunke}
\author[c]{Glenn Flierl}
\author[d]{Sebastian D. Eastham}
\author[b,c,e]{Noelle E. Selin}

\affil[a]{Department of Aeronautics and Astronautics, \authorcr Massachusetts Institute of Technology, Cambridge, MA, United States}
\affil[b]{Center for Sustainability Science and Strategy, \authorcr Massachusetts Institute of Technology, Cambridge, MA, United States}
\affil[c]{Department of Earth, Atmospheric, and Planetary Sciences, \authorcr Massachusetts Institute of Technology, Cambridge, MA, United States}
\affil[d]{Brahmal Vasudevan Institute for Sustainable Aviation, Department of Aeronautics, \authorcr Imperial College London, London, United Kingdom}
\affil[e]{Institute for Data, Systems, and Society, \authorcr Massachusetts Institute of Technology, Cambridge, MA, United States}
\date{}

\begin{document}
\maketitle

\tableofcontents
\clearpage

%\appendix
\renewcommand{\thetable}{S\arabic{table}}
\renewcommand{\thefigure}{S\arabic{figure}}
\renewcommand{\thealgorithm}{S\arabic{algorithm}}
\renewcommand{\thesubsection}{\thesection.\Alph{subsection}}

In Section \ref{sec:optimization}, we describe our methodology for optimizing emulator training data by backpropagating through a differentiable model, beginning with a conceptual example to motivate our procedure. We then outline the development of a Python-based differentiable \gls{scm} using the JAX numerical library in Section \ref{sec:scm}, including descriptions of the model's structure and gradient-based calibration procedure. In Section \ref{sec:emulator}, we present a neural network emulator of our \gls{scm}, highlighting its architecture, feature design, and training procedure. In Section \ref{sec:mesm}, we describe how we extend the training data optimization process and emulator creation to the \gls{mesm}, followed by an outline of the scenarios and metrics used during evaluation in Section \ref{sec:evaluation}. We conclude with sensitivity analyses for our optimization procedure (Section \ref{sec:sensitivity}) and extended results from the main manuscript (Section \ref{sec:ex_results}).

\section{Training data optimization}\label{sec:optimization}

\subsection{Conceptual overview}\label{sec:concept}
We use the following problem of estimating unknown linear system parameters as a conceptual example to motivate our optimization procedure. It does not extend directly to our full system because the full system is nonlinear, state dependent, and our full system objective is predictive skill over some set of metrics, rather than parameter estimation. Despite this, the linear system is highly useful because it is interpretable, enabling us to better understand our optimization requirements.

Consider emulating a discrete, linear system via explicit parameter estimation. For example, estimating climate sensitivity and carbon uptake terms for a simple climate model to predict global mean temperature anomaly from CO$_2$ emissions. Our goal is to determine the set of training data that maximizes the accuracy of our parameter estimates. The system of interest is given by
\begin{equation}
    \bT_{n+1} = \bN \bT_n + \bu_n,
\end{equation}
where $\bT$ is the temperature, $\bN$ is the linear operator that evolves the temperature forward in time, and $\bu$ is a known forcing (e.g., emissions). We can emulate this system by estimating the parameters of $\bN$ and using the recovered operator to step our system forward in time from some initial condition. We use standard dynamic mode decomposition \cite{schmid_dynamic_2010} to estimate $\bN$ via least squares as
\begin{equation}
    \tilde{\bN} \approx \left[\bT_{n+1} - \bu_n\right]\bT_n^{\dagger},
\end{equation}
where $\dagger$ indicates the Moore-Penrose pseudoinverse.

The accuracy of the estimate of $\bN$ is controlled by the conditioning of the training data: the forcing $\bu_n$ and the resulting temperature trajectory $\bT_n(\bu_n)$. If the chosen forcing is uninformative (e.g., nearly constant or exponential, as in Giani et al. \cite{giani_origin_2024} and Womack et al. \cite{womack_theoretical_2026}), then the columns of the data matrix constructed from $\bT_n$ become nearly collinear. In the more realistic case where we only observe noisy states $\tilde{\bT} = \bT + \varepsilon$, where $\varepsilon$ corresponds to some measurement error or stochastic noise (e.g., internal variability), the error in our estimated operator $\tilde{\bN}$ is bounded by the condition number, $\kappa$, of the data matrix:
\begin{equation}
    \frac{||\tilde{\bN} - \bN||}{||\bN||} \lesssim \kappa(\bT_n) \frac{||\varepsilon||}{||\bT_n||}.
\end{equation}
Here, $\kappa(\bT_n)$ acts as an amplification factor. If the data are ill-conditioned ($\kappa \gg 1$), even a small amount of noise leads to large errors in the learned dynamics. As a result, designing the forcing $\bu_n$ becomes a problem of optimal experimental design \cite{fedorov_optimal_2010}. We aim to find the forcing $\bu^*$ that minimizes this error bound:
\begin{equation}
    \bu^* = \argmin_\bu \kappa(\bT_n(\bu)).
\end{equation}
If the map $\bu \mapsto \bT(\bu)$ is differentiable, we can, in principle, compute $\nabla_\bu \kappa$ and use gradient descent to iteratively update $\bu$ so that the resulting temperature response is maximally informative for parameter estimation. 

While minimizing the condition number is optimal for linear parameter recovery, this approach breaks down for our full-scale system. In general, manually deriving and implementing an adjoint model of a system of interest to calculate gradients is intractable due to its complexity (e.g., \glspl{esm} written in Fortran with millions of lines of code). To address this, we generalize the logic above to leverage backpropagation to calculate gradients. 

\subsection{Framework for training data optimization}\label{sec:backprop}

We frame the generation of training data as a bi-level optimization problem. Rather than designing an explicit adjoint model, we utilize \gls{ad}. \gls{ad} allows us to accurately and efficiency compute derivatives of complex functions by leveraging the chain rule through the computational graph. This technique is preferable to traditional numerical methods (e.g., finite differences) as it incurs a lower computational cost and computes exact derivatives.

Our objective is to find a specific set of training emissions $\bU_\text{train}$ that minimizes the error of an emulator trained on that data when tested against a held-out target set. This problem consists of an implicit inner level (training the emulator parameters $\theta$ using $\bU_\text{train}$) and an explicit outer level (updating $\bU_{\text{train}}$ to minimize the test loss of the trained emulator). The optimization objective is given mathematically as
\begin{equation}
    \operatorname*{\argmin}_{\bU_\text{train}} \cL_{\text{test}}(\bU_\text{train}, \, \theta_\text{train}, \, D_{\text{test}}),
\end{equation}
where $\theta_\text{train}$ represents the parameters of the emulator after training on the data generated by $\bU_\text{train}$. While this methodology is generalizable to models of other physical systems, we apply it here to an \gls{scm}. The procedure is detailed below, with Algorithm \ref{alg:opt} providing a summary; also see Figs. 1 and 2 in the main text for an overview of the optimization process and illustrative example, respectively.

\textbf{Inner level.} The inner level of the optimization consists of training an emulator to map from emissions to temperature anomalies. The process is defined by the following:
\begin{enumerate}
    \item Emissions training data ($\bU_\text{train} \in \mathbb{R}^{n_\text{agents} \times n_t}$): The trainable parameters are a collection of emission time series for $n_\text{agents}$ forcing agents (e.g., CO$_2$, CH$_4$, etc.) over $n_t$ time steps.
    \item Training features ($\bX_{\text{train}} \in \mathbb{R}^{n_t \times d}$): We construct features from $\bU_\text{train}$ using instantaneous emissions, cumulative emissions, and exponential moving averages for each forcing agent. The resulting features are dimension $d=n_\text{agents} \times n_\text{feat.}$, where $n_\text{feat.}$ is equal to the number of features per agent.
    \item Training targets ($\overline{\Delta T}(t) = \by_\text{train} \in \mathbb{R}^{n_t}$): We force the \gls{scm} with $\bU_\text{train}$ to generate the corresponding \gls{gmst} anomalies, which serve as ground-truth targets. 
    \item Inner optimization: The emulator (a neural network with parameters $\theta$) is trained to minimize the \gls{mse} between its predictions and $\by_\text{train}$. Starting from initial weights $\theta_0$, we perform $k$ steps of \gls{sgd}: 
    \begin{equation}
        \theta_k = \text{SGD}(\theta_0; \, \bX_\text{train}, \, \by_\text{train}, \, k).
    \end{equation}
\end{enumerate}

\clearpage

\textbf{Outer level.} The outer level tests the performance of the trained emulator with parameters $\theta_k$ on a dataset held constant during optimization, and backpropagates the error through the test, training, and data generation steps to update $\bU_\text{train}$. The process is defined by the following:

\begin{enumerate}
    \item Test loss ($\cL_\text{test}$): The trained emulator is tested on a fixed set of scenarios ($\bX_\text{test}, \by_\text{test}$), constructed from prescribed emissions independent of $\bU_\text{train}$. However, to ensure consistency, both train and test features are normalized using summary statistics (mean and variance) computed from the current training features $\bX_\text{train}$. We quantify test performance using \gls{nrmse}, weighted by scenario length and averaged across $N_\text{scen}$ test scenarios:
    \begin{equation}\label{eq:NRMSE}
        \cL_\text{test} = \frac{1}{N_\text{scen}}\sum_{i=1}^{N_\text{scen}}w_i\frac{\text{RMSE}\left(f\left(\bX^{(i)}_\text{test}; \, \theta_k\right), \, \by^{(i)}_\text{test}\right)}{\max_t |\by^{(i)}_\text{test}(t)|},
    \end{equation}
    where $f$ denotes the emulator and $w_i$ accounts for the relative length of scenario $i$.
    \item Gradient calculation: We update $\bU_\text{train}$ to minimize $\cL_\text{test}$. By the chain rule, the gradient $\partial\mathcal{L}_{\text{test}}/\partial\bU_\text{train}$ is decomposed as
    \begin{equation}
        \PD{\cL_\text{test}}{\bU_\text{train}} = \underbrace{\PD{\cL_\text{test}}{\theta_k} \cdot \PD{\theta_k}{\bU_\text{train}}}_\text{Parameter sensitivity} + \underbrace{\PD{\mathcal{L}_\text{test}}{\mathbf{X}_\text{test}} \cdot \PD{\mathbf{X}_\text{test}}{\bU_\text{train}}}_\text{Normalization sensitivity}.
    \end{equation}
    The first term captures how changing emissions alters the trained model parameters. The second term accounts for the dependence of the feature normalization statistics (mean and variance) on the training data $\bU_\text{train}$. The parameter sensitivity is then expanded further:
    \begin{equation}
        \PD{\theta_k}{\bU_\text{train}} = \underbrace{\PD{\theta_k}{\bX_\text{train}} \cdot \PD{\bX_\text{train}}{\bU_\text{train}}}_\text{Feature sensitivity} + \underbrace{\PD{\theta_k}{\by_\text{train}} \cdot \PD{\by_\text{train}}{\bU_\text{train}}}_\text{Physics sensitivity}.
    \end{equation}
    Here, $\partial \by_{\text{train}}/\partial \bU_\text{train}$ requires differentiating through the \gls{scm} physics, while $\partial \bX_{\text{train}}/\partial \bU_\text{train}$ involves differentiating through the feature engineering operations (e.g., moving averages). We rely on \gls{ad} to propagate these gradients through the full pipeline.
    \item Emissions update: At iteration $n$, we update the emissions using the computed gradient:
    \begin{equation}
        \bU_{n+1} = \bU_n - \eta \nabla_{\bU_\text{train}} \cL_\text{test},
    \end{equation}
    where $\eta$ is the learning rate. In practice, a different learning rate is applied to each forcing agent, as the magnitude of the gradient with respect to each agent can vary by several orders of magnitude. The final updates are applied via an \gls{sgd} optimizer with momentum \cite{liu_improved_2020} to yield a locally optimal emissions trajectory $\bU^*$.
\end{enumerate}

\begin{algorithm}[ht]
\caption{Bi-level training data optimization procedure. The inner loop trains the emulator parameters $\theta$ while the outer loop tests performance and updates the training emissions $\bU_\text{train}$.}\label{alg:opt}
\begin{algorithmic}[1]
\Require $\bU_\text{train}$ (initial emissions), $\bX_\text{test}, \by_\text{test}$ (test set), $\theta_0$ (initial weights)
\Statex
\While{not converged}
    \State \textcolor{gray}{\# 1. Data generation \& feature engineering}
    \State $\by_\text{train} = \text{SCM}(\bU_\text{train})$ 
    \State $\bX_\text{train} = \text{Featurize}(\bU_\text{train})$
    \State $\mu_\text{train}, \, \sigma_\text{train} = \text{get\_stats}(\bX_\text{train})$ \Comment{Compute normalization statistics from training data}
    \State $\bX_\text{train}^{\text{norm}} = (\bX_\text{train} - \mu_\text{train}) / \sigma_\text{train}$
    \Statex
    \State \textcolor{gray}{\# 2. Inner loop: Emulator training}
    \State $\theta = \theta_0$ \Comment{Reset weights completely before training}
    \For{$k$ in $\text{range}(K)$} \Comment{$K = $ number of training gradient descent steps}
        \State $\hat{\by} = f(\bX_\text{train}^{\text{norm}}; \, \theta)$
        \State $\cL_\text{train} = \text{MSE}(\hat{\by}, \, \by_\text{train})$
        \State $\theta = \text{SGD}(\theta, \, \nabla_\theta \cL_\text{train})$ \Comment{Update weights}
    \EndFor
    \Statex
    \State \textcolor{gray}{\# 3. Outer loop: Test \& update}
    \State $\bX_\text{test}^{\text{norm}} = (\bX_\text{test} - \mu_\text{train}) / \sigma_\text{train}$ \Comment{Normalize test data using training stats}
    \State $\hat{\by}_\text{test} = f(\bX_\text{test}^{\text{norm}}; \, \theta)$
    \State $\cL_\text{test} = \text{NRMSE}(\hat{\by}_\text{test}, \by_\text{test})$ \Comment{Compute weighted test loss (Eq. \ref{eq:NRMSE})}
    \Statex
    \State $\text{grads} = \nabla_{\bU_\text{train}} \cL_\text{test}$ \Comment{Backpropagate through testing, training, and physics via \gls{ad}}
    \State $\bU_\text{train} = \text{Optimizer}(\bU_\text{train}, \, \text{grads})$ \Comment{Update emissions via \gls{sgd} with momentum}
\EndWhile
\State \Return $\bU_\text{train}$
\end{algorithmic}
\end{algorithm}

\clearpage

\section{Differentiable simple climate model}\label{sec:scm}

To enable the optimization procedure outlined in Section \ref{sec:optimization}, we present a differentiable simple climate model that calculates annual-average \gls{gmst} anomalies based on the \gls{fair} framework \cite{leach_fairv200_2021}. Implemented in JAX, this model leverages automatic differentiation to facilitate efficient gradient-based calibration.

\subsection{Model structure}

Our model retains the core structural components of \gls{fair}; see Leach et al. \cite{leach_fairv200_2021} Section 2 for a full model description. We represent the carbon cycle with a four-reservoir model, where each reservoir has an uptake fraction and a decay timescale. These reservoirs are mathematical abstractions representing the different timescales of carbon removal---ranging from rapid biospheric uptake to slow geological weathering---rather than distinct physical stores (e.g., the deep ocean). The decay time constants are scaled by a state-dependent feedback parameter, $\alpha$. This factor incorporates nonlinear feedbacks, such as the saturation of carbon sinks, based on cumulative carbon uptake and \gls{gmst} anomalies. We calculate temperature anomalies using a three-box impulse response model based on total effective radiative forcing from forcing agent concentrations. This component accounts for the thermal inertia of the climate system, capturing the delay between radiative forcing and warming caused by heat uptake in the upper and deep ocean.

We consider a subset of the forcing agents from \gls{fair}: CO$_2$, CH$_4$, N$_2$O, sulfur and \gls{bc}. We exclude minor anthropogenic gases (e.g., CFCs, HFCs) and natural forcings (solar irradiance and volcanic aerosols) to focus on the dominant drivers of future warming while retaining a tractable parameter space. For CH$_4$, and N$_2$O, we use the same governing decay equations as CO$_2$, but model them with a single reservoir. This single-reservoir approach is sufficient to capture their atmospheric residence times without the complex multi-timescale dynamics required for CO$_2$. CH$_4$ retains a state-dependent lifetime calculation similar to CO$_2$ (dependent on temperature and atmospheric burden), while N$_2$O is modeled with a constant lifetime. Finally, we assume sulfur and black carbon emissions directly impact effective radiative forcing through aerosol-radiation and aerosol-cloud interactions, following the parameterization in Leach et al. \cite{leach_fairv200_2021}.

\subsection{Model calibration}\label{sec:calibration}

We use automatic differentiation to enable gradient-based calibration, calibrating our model to reproduce the temperature response of the \gls{fair} model. To establish a ground-truth target, we configure \gls{fair} using the median parameters values from the probabilistic ensemble derived in Smith et al. \cite{smith_faircalibrate_2024}, which was constrained to reproduce climate responses based on \glspl{esm} from \gls{cmip6} or \gls{ipcc}-assessed ranges. To isolate the response of each forcing agent for calibration, we use single-forcing experiments generated from the \gls{cmip7} ScenarioMIP\footnote{At the time of performing this investigation and writing this manuscript, the final version of ScenarioMIP-CMIP7 was not yet published. As a result, we use the scenarios outlined in the preprint manuscript, not including the \textit{High-to-Low} scenario added in the final version.} and DECK protocols \cite{vanvuuren_scenario_2026, dunne_evolving_2025}; for forcing agents without single-forcing experiments in the DECK, we prescribe protocols equivalent to \textit{abrupt-4xCO2} and \textit{1pctCO2} (e.g., \textit{abrupt-4xCH4} and \textit{1pctN2O}). A full list of calibration experiments can be found in Table \ref{tab:scenarios}.

Unlike the standard \gls{fair} calibration methodology, which employs a Bayesian framework to generate a posterior distribution of parameters \cite{smith_faircalibrate_2024}, we perform deterministic parameter estimation via gradient-based optimization. Using the Adam optimizer \cite{kingma_adam_2017}, we minimize \gls{nrmse} between our model's \gls{gmst} and the \gls{fair} reference outputs over the simulation period. We use \gls{nrmse} to handle the disparate scales of temperature anomalies across scenarios (e.g., 6$^\circ$C in \textit{abrupt-4xCO2} vs. $< 2^\circ$C in \textit{VLLO}), normalizing by the range of the reference temperature trajectory (Equation \ref{eq:NRMSE}). This normalization ensures equal weighting across scenarios, preventing high-warming trajectories from dominating the loss function. We conduct calibration sequentially by agent and component (e.g., separating carbon cycle parameters from thermal response parameters), utilizing gradient masking to freeze non-target parameters during each stage.

\section{Neural network emulator}\label{sec:emulator}

We implement a neural network emulator for the differentiable \gls{scm} outlined in Section \ref{sec:scm} that predicts \gls{gmst} from emissions. This component serves as a proof-of-concept to demonstrate that the differentiable framework functions as intended to optimize training data (Section \ref{sec:optimization}).

We employ a lightweight architecture (emulator structure) designed to minimize computational burden while maintaining sufficient fidelity to map emissions to temperature response. While more complex deep learning architectures (e.g., LSTMs or Transformers) could yield higher predictive skill, our objective is to isolate the effect of training data composition rather than model complexity. As a result, we prioritize training speed; all training reported here was completed on a standard laptop CPU (MacBook Pro, M1 Chip).

\subsection{Feature design and architecture}

To capture the temporal dynamics and inertia of the climate system without the computational cost and complexity of an autoregressive model, we construct a feature vector that implicitly encodes the atmospheric state and memory of past forcings. For a given simulation year $t$, the input vector $\bX_t$ summarizes the history of emissions up to year $t-1$. For each forcing agent, we calculate five scalar features (1) the emissions at the previous timestep; (2) the cumulative emissions to date; and (3) \glspl{ema} of the emissions calculated with decay timescales of five, thirty, and one hundred years. These timescales were selected to approximate the multiple response timescales of the carbon cycle and thermal response.

These features are fed into a standard \gls{mlp}. The network consists of a single hidden layer with hyperbolic tangent ($\tanh$) activations, followed by a linear output layer that predicts the scalar \gls{gmst} anomaly for year $t$. Prior to training, all input features are standardized to zero mean and unit variance.

\subsection{Training}

We train the emulator to predict \gls{gmst} by minimizing the \gls{mse} between the emulator predictions and the true \gls{scm} output. Note this training loss (\gls{mse}) is distinct from the \gls{nrmse} used in the outer optimization level. We train distinct emulator configurations to compare the impact of training data on predictive skill. To ensure fair comparison, we use a consistent number of gradient training steps for all emulator configurations, regardless of the size or composition of the training dataset.

\textbf{Baseline emulator.} We train the baseline emulator on Priority 1 scenarios from \gls{cmip7} ScenarioMIP protocol \cite{vanvuuren_scenario_2026}. We selected this baseline as it represents the standard set of scenarios that all modeling centers are expected to generate, ensuring broad accessibility.

\textbf{Optimized emulator.} The optimized emulator utilizes an identical architecture, feature set, and training hyperparameters (e.g., learning rate) as the baseline, but is trained on the synthetic datasets generated via the optimization process described in Section \ref{sec:optimization}.

\section{Extension to the MIT Earth System Model}\label{sec:mesm}
We apply our framework to \gls{mesm} to demonstrate its scalability and utility for generating informative training datasets even when the target model is not differentiable. \gls{mesm} is a zonally averaged \gls{emic} that includes a two-dimensional, zonally averaged atmospheric model with interactive chemistry coupled to a zonally averaged land model and an anomaly-diffusing ocean model; see Sokolov et al. \cite{sokolov_description_2018} for a full description. As \gls{mesm} is not differentiable, we recalibrate the differentiable \gls{scm} to act as a surrogate for \gls{mesm}.

We recalibrate the \gls{scm} to approximate the \gls{mesm} temperature response in two stages, using CO$_2$-only scenarios. First, we constrain the climate sensitivity parameters (thermal response) by minimizing the loss between \gls{scm} and \gls{mesm} \gls{gmst} anomalies under scenarios with prescribed CO$_2$ concentrations (e.g., \textit{1pctCO2}). Then, we calibrate the carbon cycle parameters using emissions-driven scenarios, minimizing the error in simulated atmospheric CO$_2$ concentrations. To filter \gls{mesm}'s internal variability, we target the mean of a thirty-member initial condition ensemble for all components of calibration, optimization, and emulation.

We assume that the training data optimized for this \gls{mesm}-tuned \gls{scm} will be highly informative for training an emulator of the actual \gls{mesm}. This approach relies on the assumption that loss landscape topology of the recalibrated \gls{scm} is sufficiently similar to that of \gls{mesm}, allowing gradients computed through the \gls{scm} to guide data selection for the more complex model.

Following recalibration, we utilize the bi-level optimization procedure using the \gls{scm} to generate optimized emissions trajectories. We then evaluate these datasets by training a new emulator for \gls{mesm}. Unlike the global-mean emulator outlined in the previous section, this emulator is modified to predict zonal temperature anomalies by modifying the output layer of the neural network to produce a vector (predictions at each latitude band), rather than a scalar; the feature generation remains the same. We benchmark the performance of the emulators trained on our optimized datasets against a baseline emulator trained on ScenarioMIP Priority 1 scenarios, evaluating all emulators on the remaining scenarios. As the area of each latitude band is non-uniform and decreasing towards the poles, we use area-weighted error metrics during training and evaluation:
\begin{align}
    \mathcal{L}_\text{zonal}(\phi) &= \cos(\phi) \langle E\rangle_t,\\
    \mathcal{L}_\text{global} &= \frac{\sum_{\phi} \mathcal{L}_\text{zonal}(\phi)}{\sum_\phi \cos(\phi)},
\end{align}
where $\phi$ denotes the latitude, $E$ denotes the error metric of interest, and $\langle\cdot\rangle_t$ denotes the temporal average over a scenario. The error metric is \gls{mse} during training and \gls{nrmse} during evaluation, and must be normalized by the magnitude of the weights to ensure the global metric remains in the same units and scale as the zonal errors.

\section{Scenario descriptions and evaluation protocol}\label{sec:evaluation}

We use \gls{nrmse} (Equation \ref{eq:NRMSE}) as our primary evaluation metric. By normalizing RMSE by the maximum absolute magnitude of the \gls{scm}- or \gls{emic}-projected temperature trajectory, \gls{nrmse} weights all scenarios with equal importance regardless of their warming magnitude. This design choice ensures the emulator is optimized to perform well across a wide range of future pathways, rather than prioritizing high-warming scenarios where absolute errors would otherwise dominate the loss function. Table \ref{tab:scenarios} details the complete set of experiments used for calibration, optimization, and evaluation.

We compare the performance of several optimized emulator configurations against a baseline emulator, which is trained exclusively on ScenarioMIP-CMIP7 Priority 1 scenarios described in Table \ref{tab:scenarios}. For the optimized emulator, we initialize the optimization with a constant emissions trajectory and optimize for predictive skill (minimize \gls{nrmse}) over a specific test set. We optimize over up to seven different test sets, depending on if we are evaluating single-forcing or multi-forcing performance: Priority 1, Priority 2, DECK, CS3, DAMIP (multi-forcing only), GeoMIP (multi-forcing only), and All (the union of all sets). Following optimization, we evaluate the emulator's predictive skill on all other scenario sets.

To assess the emulator's generalization capability and adherence to physical principles, we include structurally distinct, out-of-distribution scenarios in our evaluation. We utilize scenarios analogous to those considered within the \gls{damip} \cite{gillett_detection_2016,gillett_detection_2025} and \gls{geomip} \cite{kravitz_geoengineering_2015} protocols. The \gls{damip}-like scenarios (\textit{Medium-GHG} and \textit{Medium-aer}) isolate the contributions of specific forcing agents by extending the \textit{historical} period into the future using the \textit{Medium} ScenarioMIP-CMIP7 scenario forcing for a subset of agents (e.g., GHGs only), while holding others constant. Similarly, the \textit{G6sulfur} scenario from \gls{geomip} introduces a stratospheric sulfate injection trajectory significantly larger than any found in standard training data, stress-testing the emulator's response to extreme aerosol forcing. Because our \gls{scm} calculates sulfur's radiative forcing contribution as parameterized aerosol-cloud interactions, the sulfur emissions of the \gls{geomip} analogue are much larger than the true \gls{geomip} protocol (i.e., unrealistic) and instead serve as a strongly out-of-distribution test for the emulator These scenarios allow us to test emulator skill in reproducing the contribution of individual forcing agents. The \textit{DECK} scenarios similarly require separation of individual forcing agents, as each experiment in the \textit{DECK} is a single-forcing experiment.

\begin{table}[b!]
\centering
\caption{Complete list of scenarios used for training, optimization, and evaluation. Scenario descriptions for ScenarioMIP are derived from the \gls{cmip7} protocol \protect\cite{vanvuuren_scenario_2026}, while CS3 scenarios are taken from the \gls{cs3}'s 2025 Global Change Outlook \cite{paltsev_2025_2025}. \textit{abrupt-4xX} and \textit{1pctX} refer to idealized single-forcing experiments performed for each agent. Scenarios containing \textit{-ext} refer to scenario extensions that end in 2500.}
\begin{tabular}{p{0.15\linewidth} p{0.2\linewidth} p{0.55\linewidth}}
\textbf{Activity} & \textbf{Scenario} & \textbf{Short Description} \\
\hline
\textbf{ScenarioMIP-CMIP7} & \textit{H-ext} & \textbf{High:} High emission scenario exploring potential high-end impacts. \\
(Priority 1) & \textit{M} & \textbf{Medium:} Medium emission scenario consistent with current policies. \\
& \textit{ML} & \textbf{Medium-Low:} Delayed mitigation effort, insufficient to meet Paris Agreement goals. \\
& \textit{L} & \textbf{Low:} Scenario consistent with likely staying below 2$^\circ$C. \\
& \textit{VLLO-ext} & \textbf{Very Low with Limited Overshoot:} Consistent with limiting warming to 1.5$^\circ$C by 2100 with limited overshoot. \\
& \textit{VLHO} & \textbf{Very Low after High Overshoot:} Scenario with similar end-of-century temperature impact to VLLO, but with delayed near-term mitigation and reliance net-negative emissions, resulting in a higher overshoot. \\
\hline
\textbf{ScenarioMIP-CMIP7} & \textit{H-ext-OS} & \textbf{High Overshoot:} Radical emissions reductions after 2100 with net zero in 2160. \\
(Priority 2) & \textit{M-ext} & Extension of the Medium scenario. \\
& \textit{ML-ext} & Extension of the Medium-Low scenario. \\
& \textit{L-ext} & Extension of the Low scenario. \\
& \textit{VLHO-ext} & Extension of the Very Low with High Overshoot scenario. \\
\hline
\textbf{DECK} & \textit{historical} & Simulation of the historical period (1850–2014) using observed forcing. \\
& \textit{abrupt-4xX} & Instantaneous quadrupling of agent $X$ (e.g., CO$_2$, CH$_4$) concentrations or emissions from pre-industrial levels. \\
& \textit{1pctX} & Concentrations or emissions of agent $X$ increase by 1\% per year until quadrupling. \\
\hline
\textbf{CS3} & \textit{CT} & \textbf{Current Trends:} Current measures for reducing greenhouse gas emissions. \\
& \textit{AA} & \textbf{Accelerated Actions:} Aggressive reductions which aim to limit and stabilize human-induced global climate warming to 1.5$^\circ$C by 2100 with a 50\% probability. \\
\hline
\textbf{DAMIP} & \textit{Medium-GHG} & Historical + Future \textit{Medium} scenario forcing for Well-Mixed GHGs only (CO$_2$, CH$_4$, N$_2$O); all other forcers held constant. \\
& \textit{Medium-aer} & Historical + Future \textit{Medium} scenario forcing for Aerosols only (Sulfur, \gls{bc}); all other forcers held constant. \\
\hline
\textbf{GeoMIP} & \textit{G6sulfur} & Stratospheric sulfur injection used to reduce \gls{gmst} from the \textit{High} (H) scenario to match that of the \textit{Medium} (M) scenario.
\end{tabular}
\label{tab:scenarios}
\end{table}

\section{Sensitivity analyses}\label{sec:sensitivity}

In this section, we examine the sensitivity of the optimization procedure to changes in the emissions \gls{ic}, neural network emulator architecture, and training features. Results in this section correspond to CO$_2$-only experiments; accompanying figures show the average performance for both the baseline and optimized emulators tested across all scenarios in the ScenarioMIP, DECK, and CS3 evaluation sets. We tune our optimization hyperparameters (e.g., gradient step size and momentum decay) to the sixteen-neuron, single-layer architecture optimized from a constant initial condition with \glspl{ema} of five, thirty, and one hundred years; this is the default configuration shown in the results of the main text. We do not necessarily expect these hyperparameters to be well-tuned for other architectures. We address the sensitivity of these hyperparameters to architectural changes where relevant.

\subsection{Sensitivity to initial condition}

Figure \ref{fig:sens_IC} illustrates the sensitivity of the optimization convergence rate and resulting emissions time series to the choice of constant, Gaussian, and sinusoidal \glspl{ic}. The final structure of the optimized emissions time series depends heavily on its initialization; all three \glspl{ic} yield distinct final trajectories. Despite this, every optimized emulator outperforms the baseline, suggesting that there exists a set of scenarios that are better suited for training than the baseline. This set is likely to be functionally infinite in size, as stochastic perturbations during optimization generate marginally different pathways for identical \glspl{ic} (not shown). Although the large-scale features of the optimized constant and Gaussian time series differ, we observe similar small-scale features, such as rapid changes in concavity. The sinusoidal emulator does not exhibit this behavior, likely because such variations are inherent to the initialization structure. Instead, the optimization targets the magnitude of each peak, breaking the symmetry of the sinusoid. While all three \glspl{ic} produce more skillful emulators than the baseline, their relative convergence rates vary. The constant \gls{ic} converges most rapidly; the sinusoidal \gls{ic} starts slowly, but approaches the skill of the constant \gls{ic} by the 1000th iteration. The Gaussian \gls{ic} yields a more skillful emulator initially, with performance on par with the baseline, but it exhibits slower overall convergence. This rate reduction is likely a consequence of the higher initial skill that results in smaller gradients. 

\subsection{Sensitivity to architecture changes}

Figures \ref{fig:sens_arch_const} and \ref{fig:sens_arch_sine} show the sensitivity of both the optimization convergence rate and resulting emissions time series to the choice of neural network architecture; the former is initialized from a constant \gls{ic} and the latter from a sinusoidal \gls{ic}. Architectural modifications alter the skill of the baseline emulator, with single-layer configurations preferable to double-layer ones. Furthermore, increasing the number of neurons in single-layer configurations improves baseline predictive skill. The constant \gls{ic} exhibits high sensitivity to architectural changes, which results in a lack of convergence relative to the primary architecture (a single hidden layer with sixteen neurons). Specifically, the optimization algorithm fails to converge for configurations with eight neurons or two layers. This failure likely stems from the gradient's sensitivity to architectural choices. Because the gradient descent hyperparameters remain fixed across architectures, they are ill-tuned for alternate configurations, leading to slow or nonexistent convergence. Conversely, the emissions time series derived from the sinusoidal \gls{ic} displays less sensitivity to architectural changes, suggesting that the gradients corresponding to this \gls{ic} are more robust to a wider range of conditions. Updates modify the magnitude of the sinusoid's peak while leaving the period nearly unchanged across all four configurations. Larger networks require additional optimization iterations to converge; this observation indicates that gradients may shrink as network size increases. The two-layer case may suffer from the converse issue of exploding gradients, evidenced by rapid error oscillations near the 100th update. This instability, likely driven by stochasticity, stabilizes quickly. Future work can incorporate results from machine learning literature regarding the origins and mitigation of such gradient issues \cite{hanin_which_2018, philipp_exploding_2018}.

\subsection{Sensitivity to features}

Figures \ref{fig:sens_feat_const} and \ref{fig:sens_feat_sine} illustrate the sensitivity of optimization convergence rate and resulting emissions time series to the choice of features; the former is initialized from a constant \gls{ic} and the latter from a sinusoidal \gls{ic}. Medium features (EMAs of thirty, fifty, and seventy years) yield superior performance for the baseline emulator, although improvement relative to long features (EMAs of fifty, one hundred, and two hundred years) is negligible. Conversely, short features (EMAs of one, five, and ten years) lead to the fastest convergence and highest skill for the constant \gls{ic} emulator. Both medium and long features exhibit slow initial convergence, suggesting that this feature-\gls{ic} combination produces small gradients. These small gradients eventually amplify to facilitate optimization convergence; the short and medium features surpass the skill of the baseline emulator for the constant \gls{ic}. As with the architectural sensitivity analysis, the sinusoidal \gls{ic} exhibits markedly lower sensitivity to the choice of features and achieves consistent convergence patterns across all three configurations. However, the initial error among the three sinusoidal emulators varies; this suggests the optimal feature set correlates with the period of the sinusoid. The structure of the resulting emissions time series varies for both \glspl{ic} across the different feature configurations. For the constant \gls{ic}, both short and medium-length features yield time series with a combination of high- and low-frequency variations. In contrast, long features result in a time series with minimal variation accompanied by the lowest rate of convergence. This behavior indicates that these features are less informative for the constant \gls{ic}. The sinusoidal case displays the opposite behavior; long features induce high-frequency changes in the optimized time series, whereas short features result in low-frequency changes. Medium features drive more consistent and substantial changes throughout the optimization process, which implies the presence of larger gradients relative to this feature set. 

\begin{figure}[!htbp]
    \centering
    \includegraphics[width=0.8\linewidth]{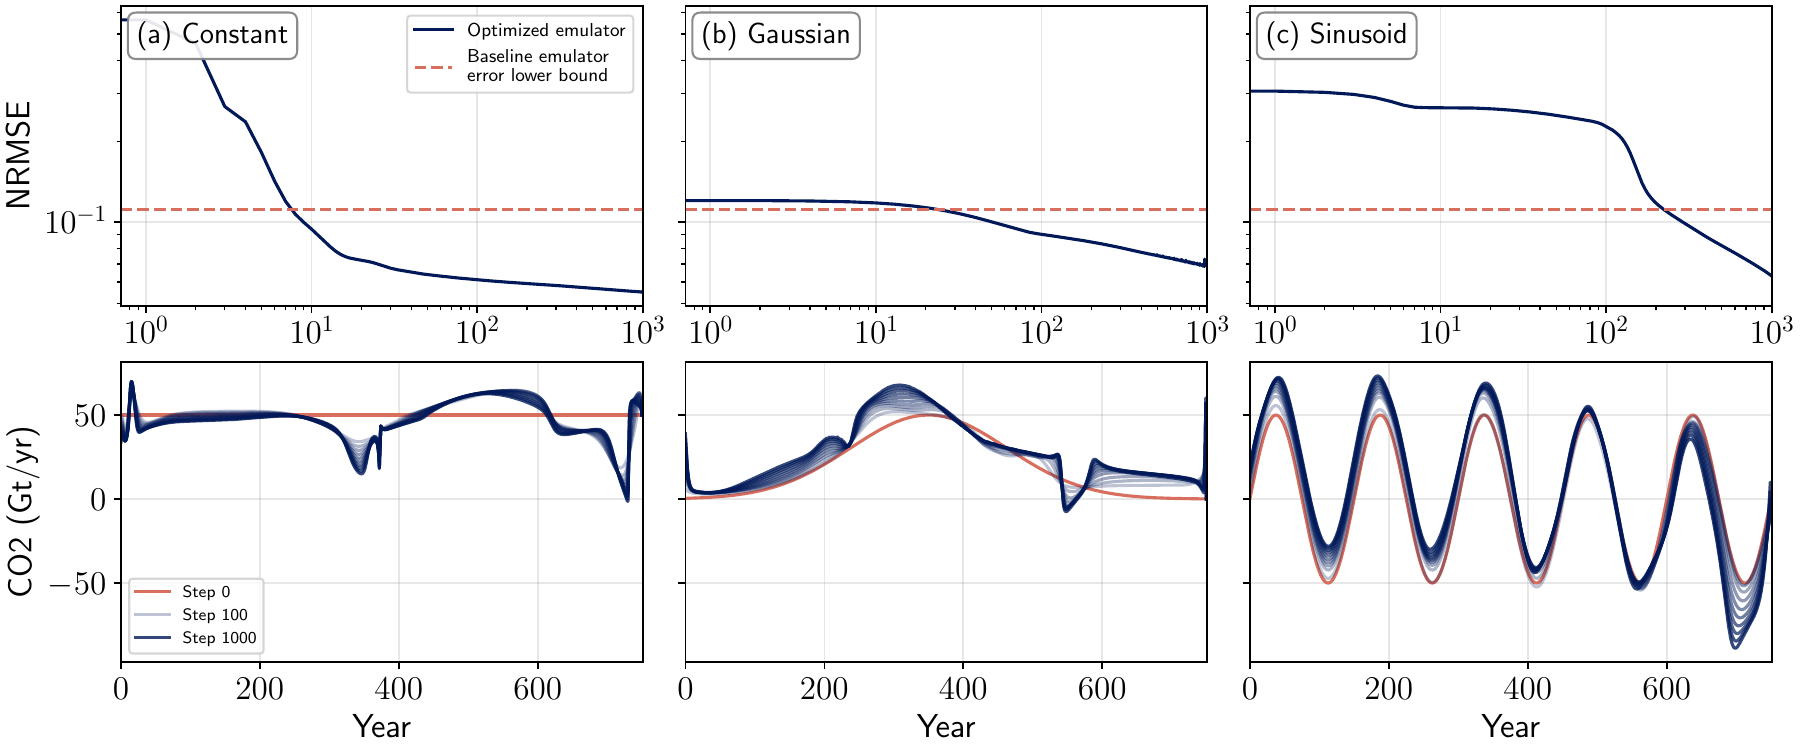}
    \caption{Top: trajectory of evaluation loss (\gls{nrmse}) during optimization compared across three \glspl{ic} for the emissions time series: (a) constant; (b) Gaussian (normally distributed in time); (c) sinusoidal with a period of 175 years. Emulators are evaluated on their performance in reproducing SCM-projected \gls{gmst} anomalies caused by CO$_2$-only across all scenarios included in the ScenarioMIP, DECK, and CS3 activities; see Table \ref{tab:scenarios} for scenario descriptions. The solid, dark blue line tracks emulator performance throughout the optimization process, while the dashed, red line marks the lower bound of the baseline emulator error (evaluating performance on its own training data). Bottom: evolution of emissions time series over 1000 iterations, corresponding to the \glspl{ic} listed above.}
    \label{fig:sens_IC}
\end{figure}

\begin{figure}[!htbp]
    \centering
    
    \includegraphics[width=\linewidth]{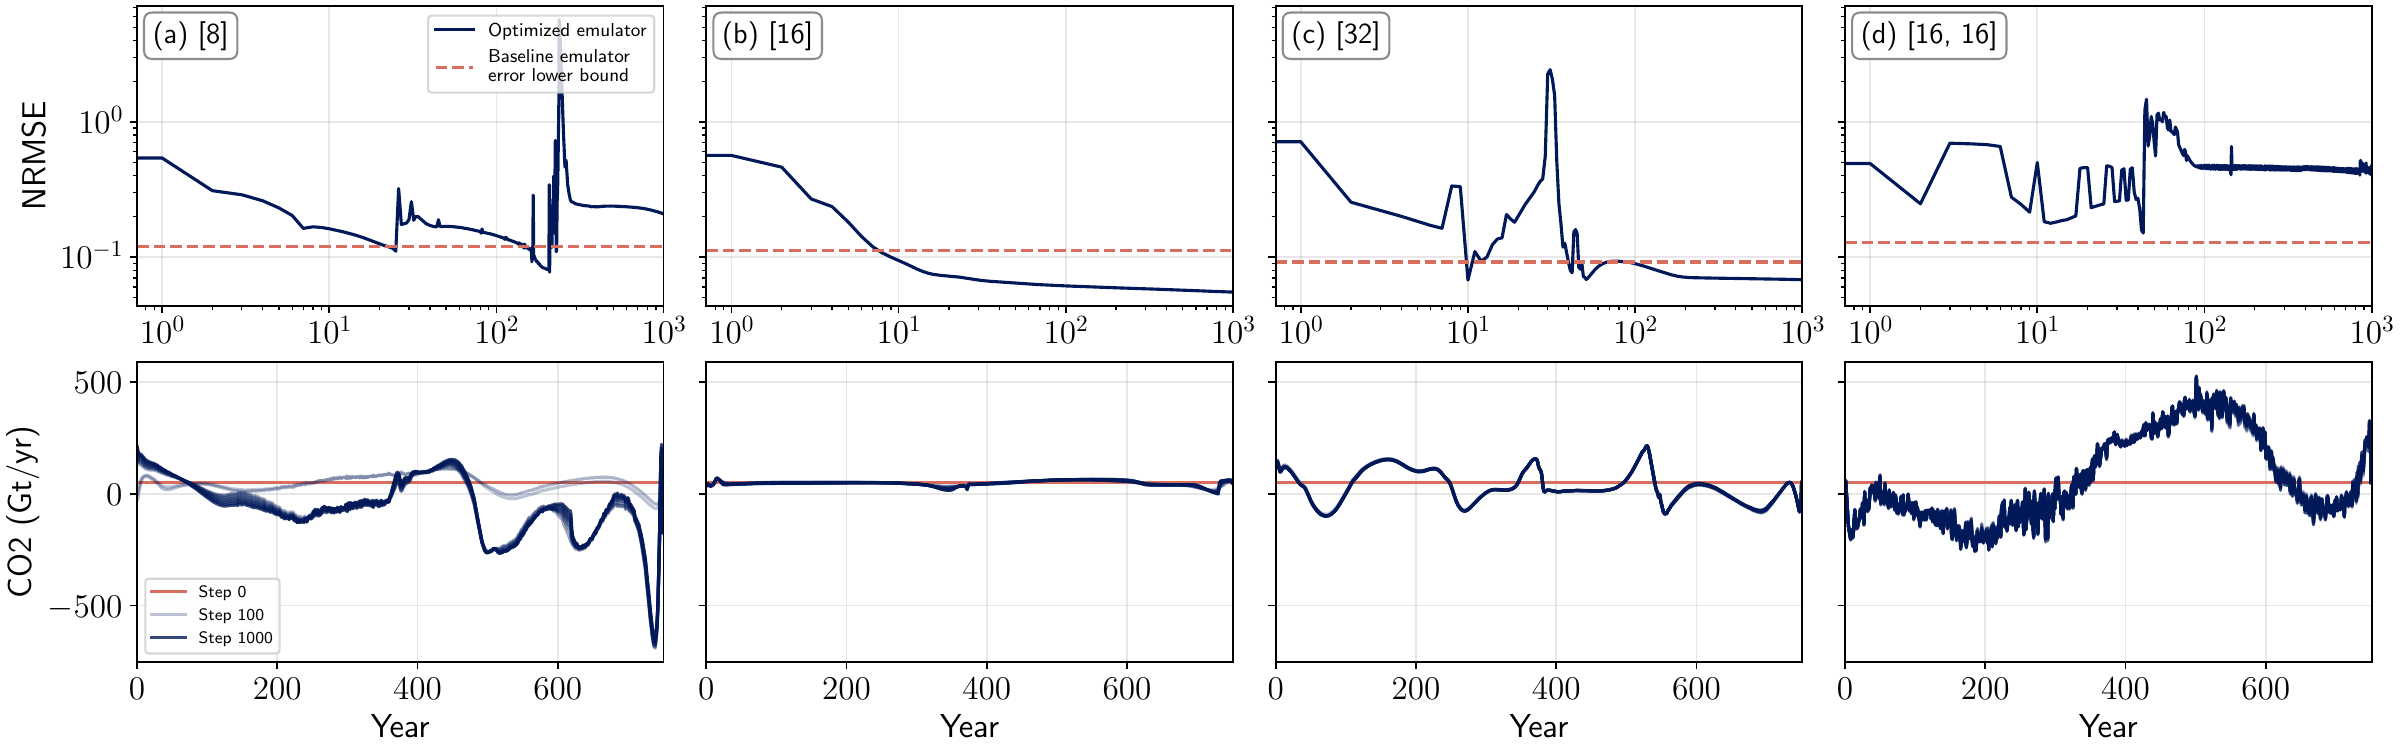}
    \caption{Top: trajectory of evaluation loss (\gls{nrmse}) during optimization compared across four architectures for the neural network emulator initialized from a constant initial condition: (a) a single hidden layer with eight neurons; (b) a single hidden layer with sixteen neurons; (c) a single hidden layer with thirty-two neurons; (d) two hidden layers with sixteen neurons each. Emulators are evaluated on their performance in reproducing SCM-projected \gls{gmst} anomalies caused by CO$_2$-only across all scenarios included in the ScenarioMIP, DECK, and CS3 activities; see Table \ref{tab:scenarios} for scenario descriptions. The solid, dark blue line tracks emulator performance throughout the optimization process, while the dashed, red line marks the lower bound of the baseline emulator error (evaluating performance on its own training data). Bottom: evolution of emissions time series over 1000 iterations, corresponding to the architectures listed above.}
    \label{fig:sens_arch_const}

    \vspace{1.5cm}

    \includegraphics[width=\linewidth]{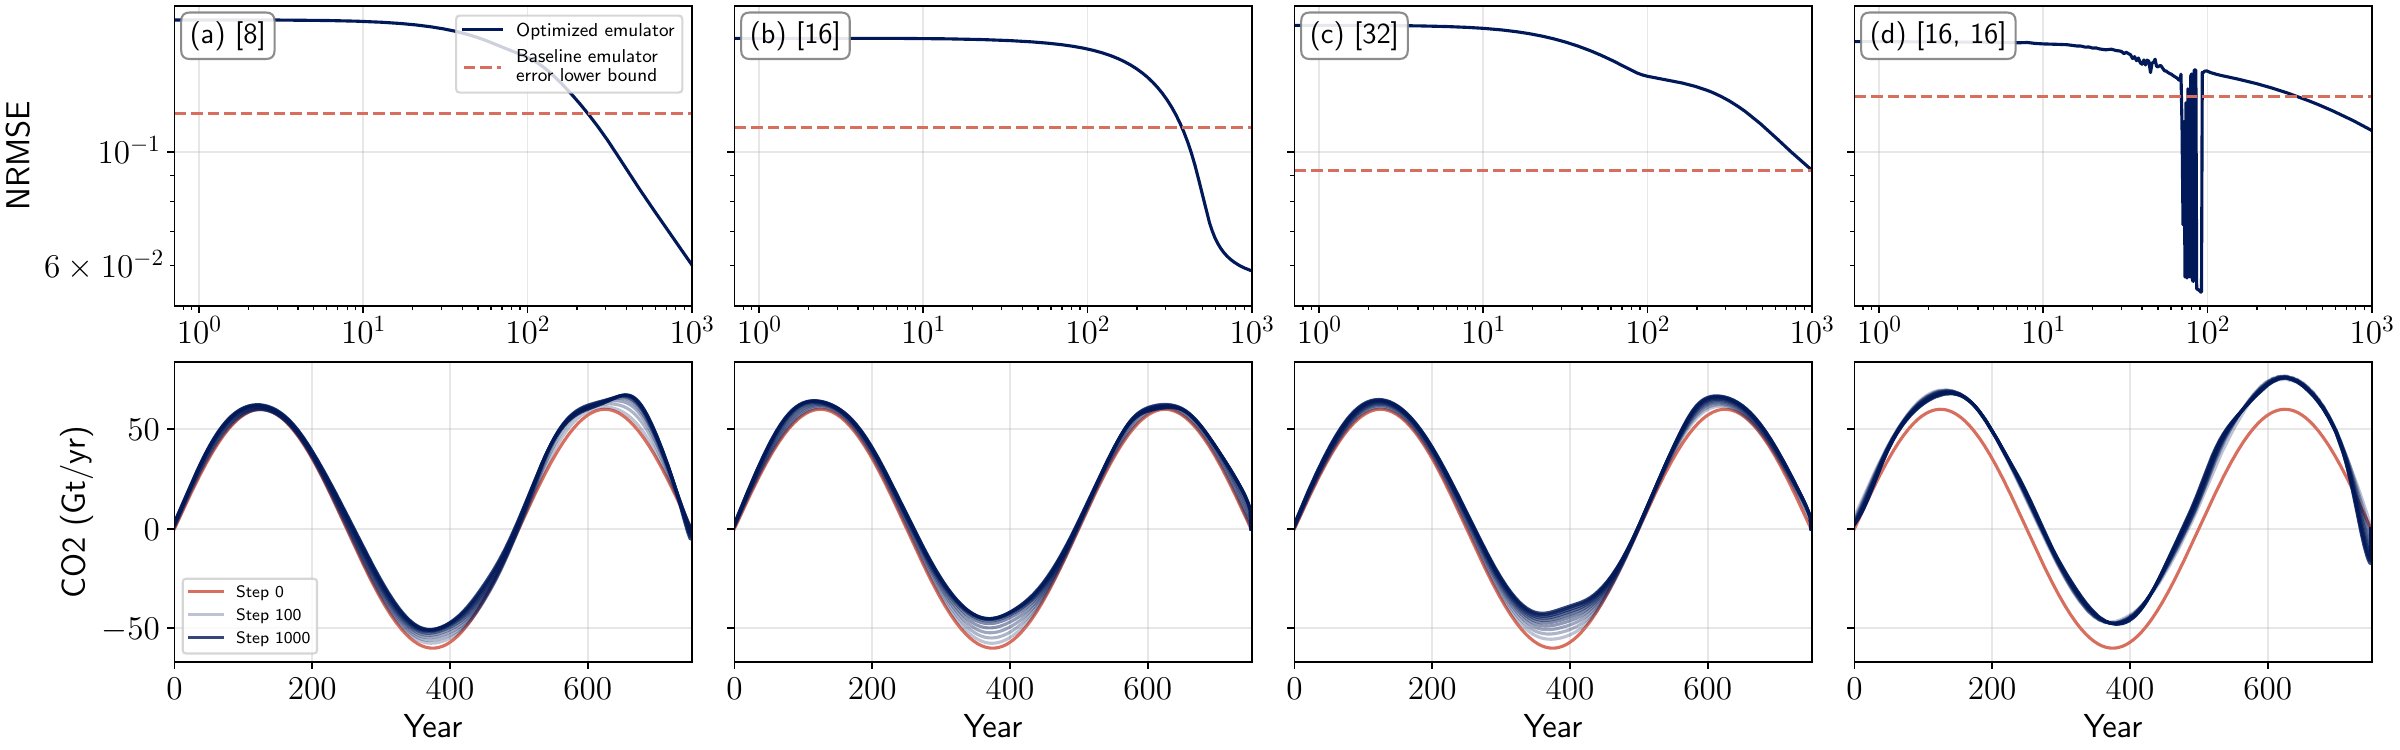}
    \caption{Top: trajectory of evaluation loss (\gls{nrmse}) during optimization compared across four architectures for the neural network emulator initialized from a sinusoidal initial condition: (a) a single hidden layer with eight neurons; (b) a single hidden layer with sixteen neurons; (c) a single hidden layer with thirty-two neurons; (d) two hidden layers with sixteen neurons each. Emulators are evaluated on their performance in reproducing SCM-projected \gls{gmst} anomalies caused by CO$_2$-only across all scenarios included in the ScenarioMIP, DECK, and CS3 activities; see Table \ref{tab:scenarios} for scenario descriptions. The solid, dark blue line tracks emulator performance throughout the optimization process, while the dashed, red line marks the lower bound of the baseline emulator error (evaluating performance on its own training data). Bottom: evolution of emissions time series over 1000 iterations, corresponding to the architectures listed above.}
    \label{fig:sens_arch_sine}
    
\end{figure}

\begin{figure}[!htbp]
    \centering
    \includegraphics[width=0.8\linewidth]{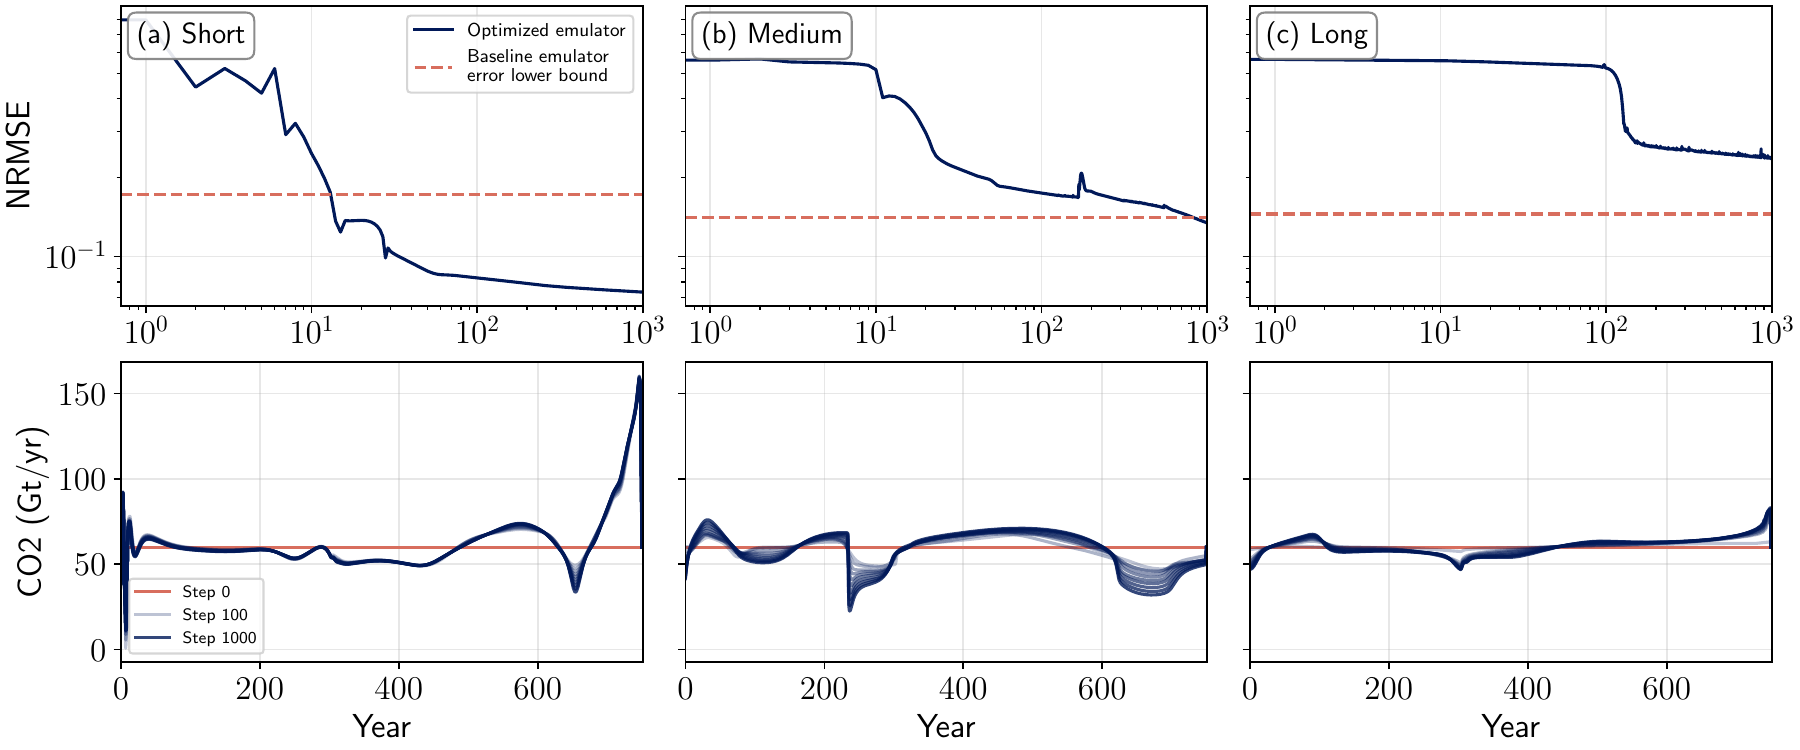}
    \caption{Top: trajectory of evaluation loss (\gls{nrmse}) during optimization compared across three sets of features for the neural network emulator initialized from a constant initial condition: (a) short - \glspl{ema} of one, five, and ten years; (b) medium - \glspl{ema} of thirty, fifty, and seventy years; (c) long - \glspl{ema} of fifty, one hundred, and two hundred years. Emulators are evaluated on their performance in reproducing SCM-projected \gls{gmst} anomalies caused by CO$_2$-only across all scenarios included in the ScenarioMIP, DECK, and CS3 activities; see Table \ref{tab:scenarios} for scenario descriptions. The solid, dark blue line tracks emulator performance throughout the optimization process, while the dashed, red line marks the lower bound of the baseline emulator error (evaluating performance on its own training data). Bottom: evolution of emissions time series over 1000 iterations, corresponding to the features listed above.}
    \label{fig:sens_feat_const}

    \vspace{1.5cm}

    \includegraphics[width=0.8\linewidth]{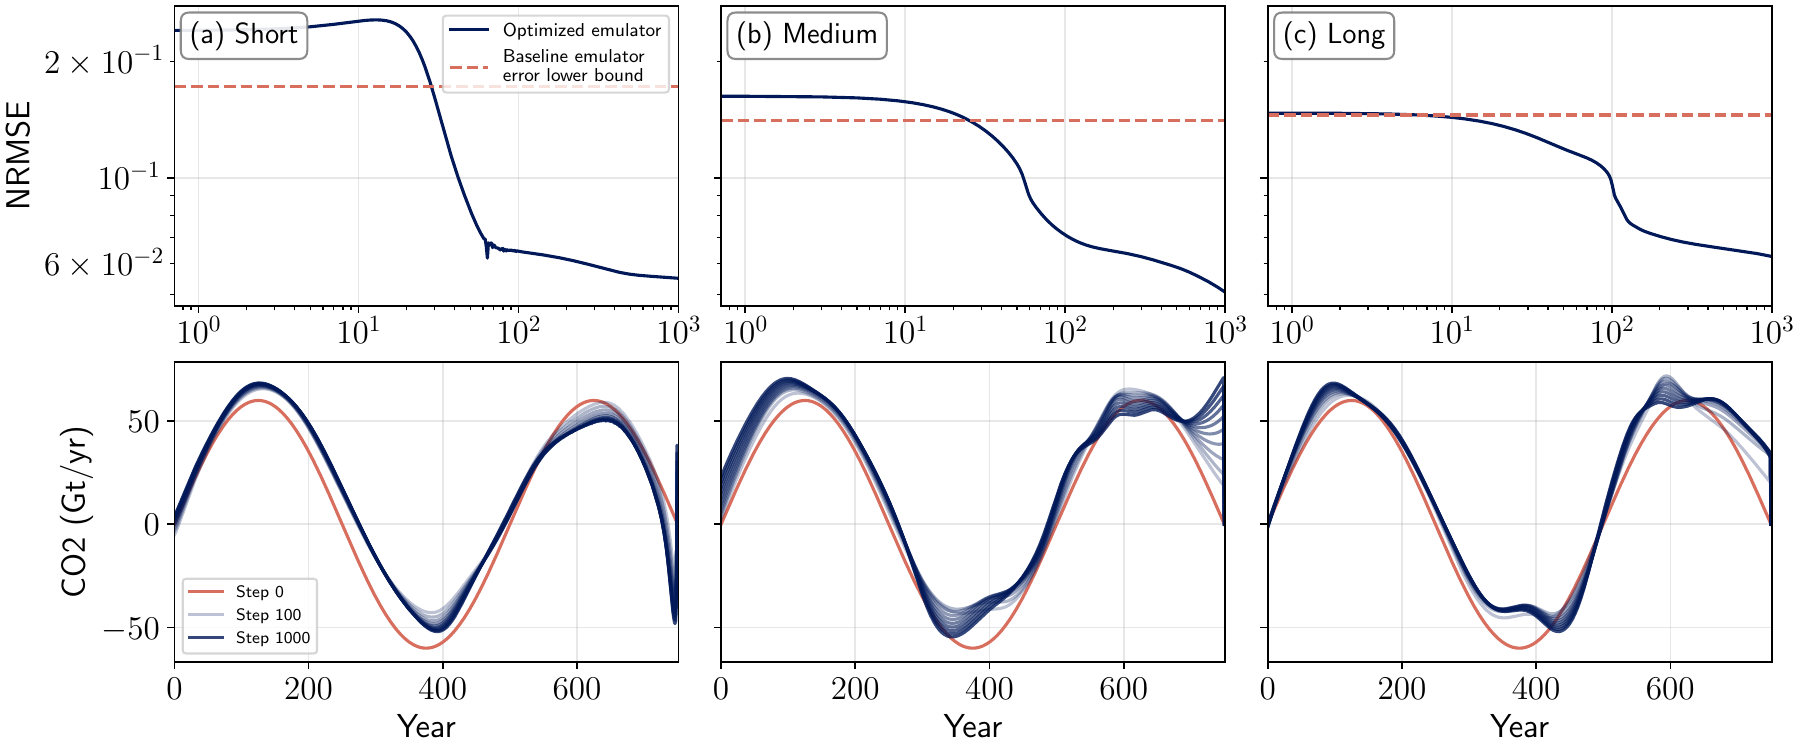}
    \caption{Top: trajectory of evaluation loss (\gls{nrmse}) during optimization compared across three sets of features for the neural network emulator initialized from a sinusoidal initial condition: (a) short - \glspl{ema} of one, five, and ten years; (b) medium - \glspl{ema} of thirty, fifty, and seventy years; (c) long - \glspl{ema} of fifty, one hundred, and two hundred years. Emulators are evaluated on their performance in reproducing SCM-projected \gls{gmst} anomalies caused by CO$_2$-only across all scenarios included in the ScenarioMIP, DECK, and CS3 activities; see Table \ref{tab:scenarios} for scenario descriptions. The solid, dark blue line tracks emulator performance throughout the optimization process, while the dashed, red line marks the lower bound of the baseline emulator error (evaluating performance on its own training data). Bottom: evolution of emissions time series over 1000 iterations, corresponding to the features listed above.}
    \label{fig:sens_feat_sine}
\end{figure}

\clearpage

\section{Extended results}\label{sec:ex_results}

Figure \ref{fig:SI_extended} summarizes the full results for the individual forcing experiments (e.g., CO$_2$-only, CH$_4$-only) introduced in the main text. While the main text provides an in-depth discussion of the CO$_2$-only results, this section focuses on the other forcing agents. The figure illustrates the difference in emulator performance between the baseline and optimized configurations; positive values indicate an increase in performance relative to the baseline, while negative values indicate a decrease. Each configuration corresponds to a different optimization target (e.g., Opt. Priority 1 corresponds to optimizing over all of ScenarioMIP-CMIP7 Priority 1).

As in the CO$_2$-only case, optimizing over all scenarios leads to increased performance over all scenarios simultaneously, rather than overfitting to a specific scenario type. However, the increase in average performance varies across forcing agents; \gls{bc} exhibits the largest improvements, whereas sulfur shows the smallest. The ability of the optimized emulators to generalize across the full set of scenario structures suggests that the training data are more informative overall. In all cases except sulfur, the optimization improves skill across Priority 1; a separate discussion of sulfur follows below. Optimizing for performance over the DECK decreases predictive skill when emulating the other scenario sets. This result is expected because the DECK scenarios are structurally dissimilar to the others. Furthermore, the small sample size (two scenarios) fails to provide the optimizer with sufficient information regarding the most generally informative features. A similar phenomenon occurs when optimizing over CS3, wherein the small number of scenarios (two) leads to overfitting and a subsequent loss of extrapolative skill for CH$_4$, N$_2$O, and sulfur. In contrast, black carbon-only scenarios show improvement in all cases. This suggests that the baseline emulator configuration is ill-suited for capturing \gls{bc} behavior. Changes to baseline emulator features and/or architecture may decrease the performance gap to the optimized emulator in this instance.

One experiment is notable within this suite: optimizing over Priority 2 in the CH$_4$-only case. Here, performance improvements relative to the baseline were unattainable on any evaluation set, a result similar to the sulfur-only experiments. Further investigation revealed two primary factors causing this result. First, the baseline emulator is well-tuned for these specific methane scenarios. Second, this optimization target is ill-conditioned for methane and exhibits high sensitivity to changes in all optimization hyperparameters. The state-dependence of atmospheric lifetime of methane may be the source of this ill-conditioning, as Priority 2 contains more long-duration scenarios than any other evaluation set. The nonlinear lifetime of methane therefore plays a larger role, and small changes in the optimized time series may lead to vastly different representations of this behavior. As a result, the optimizer oscillates between solutions and fails to find the global minimum. Despite this, adding more scenarios (i.e., optimizing over all datasets) resolves the issue, highlighting the importance of scenario diversity in the optimization process.

Although performance for the sulfur-only optimized emulator falls below the baseline more frequently than the other forcing agents, this result stems from the high skill of the baseline emulator rather than a failure of the optimization process. Unlike CO$_2$ or CH$_4$, which exhibit complex, nonlinear atmospheric residence times dependent on concentrations and temperature, forcing the \gls{scm} solely with sulfur yields temperature anomalies that are approximately linear in sulfur and respond almost instantaneously. Because this input-output mapping is structurally simple, the standard ScenarioMIP-CMIP7 baseline data already provides enough information for the emulator to learn the underlying physical relationship. As a result, the baseline emulator is effectively near its performance ceiling, leaving negligible margin for improvement via data optimization.

\begin{figure}[ht!]
    \centering
    \includegraphics[width=\linewidth]{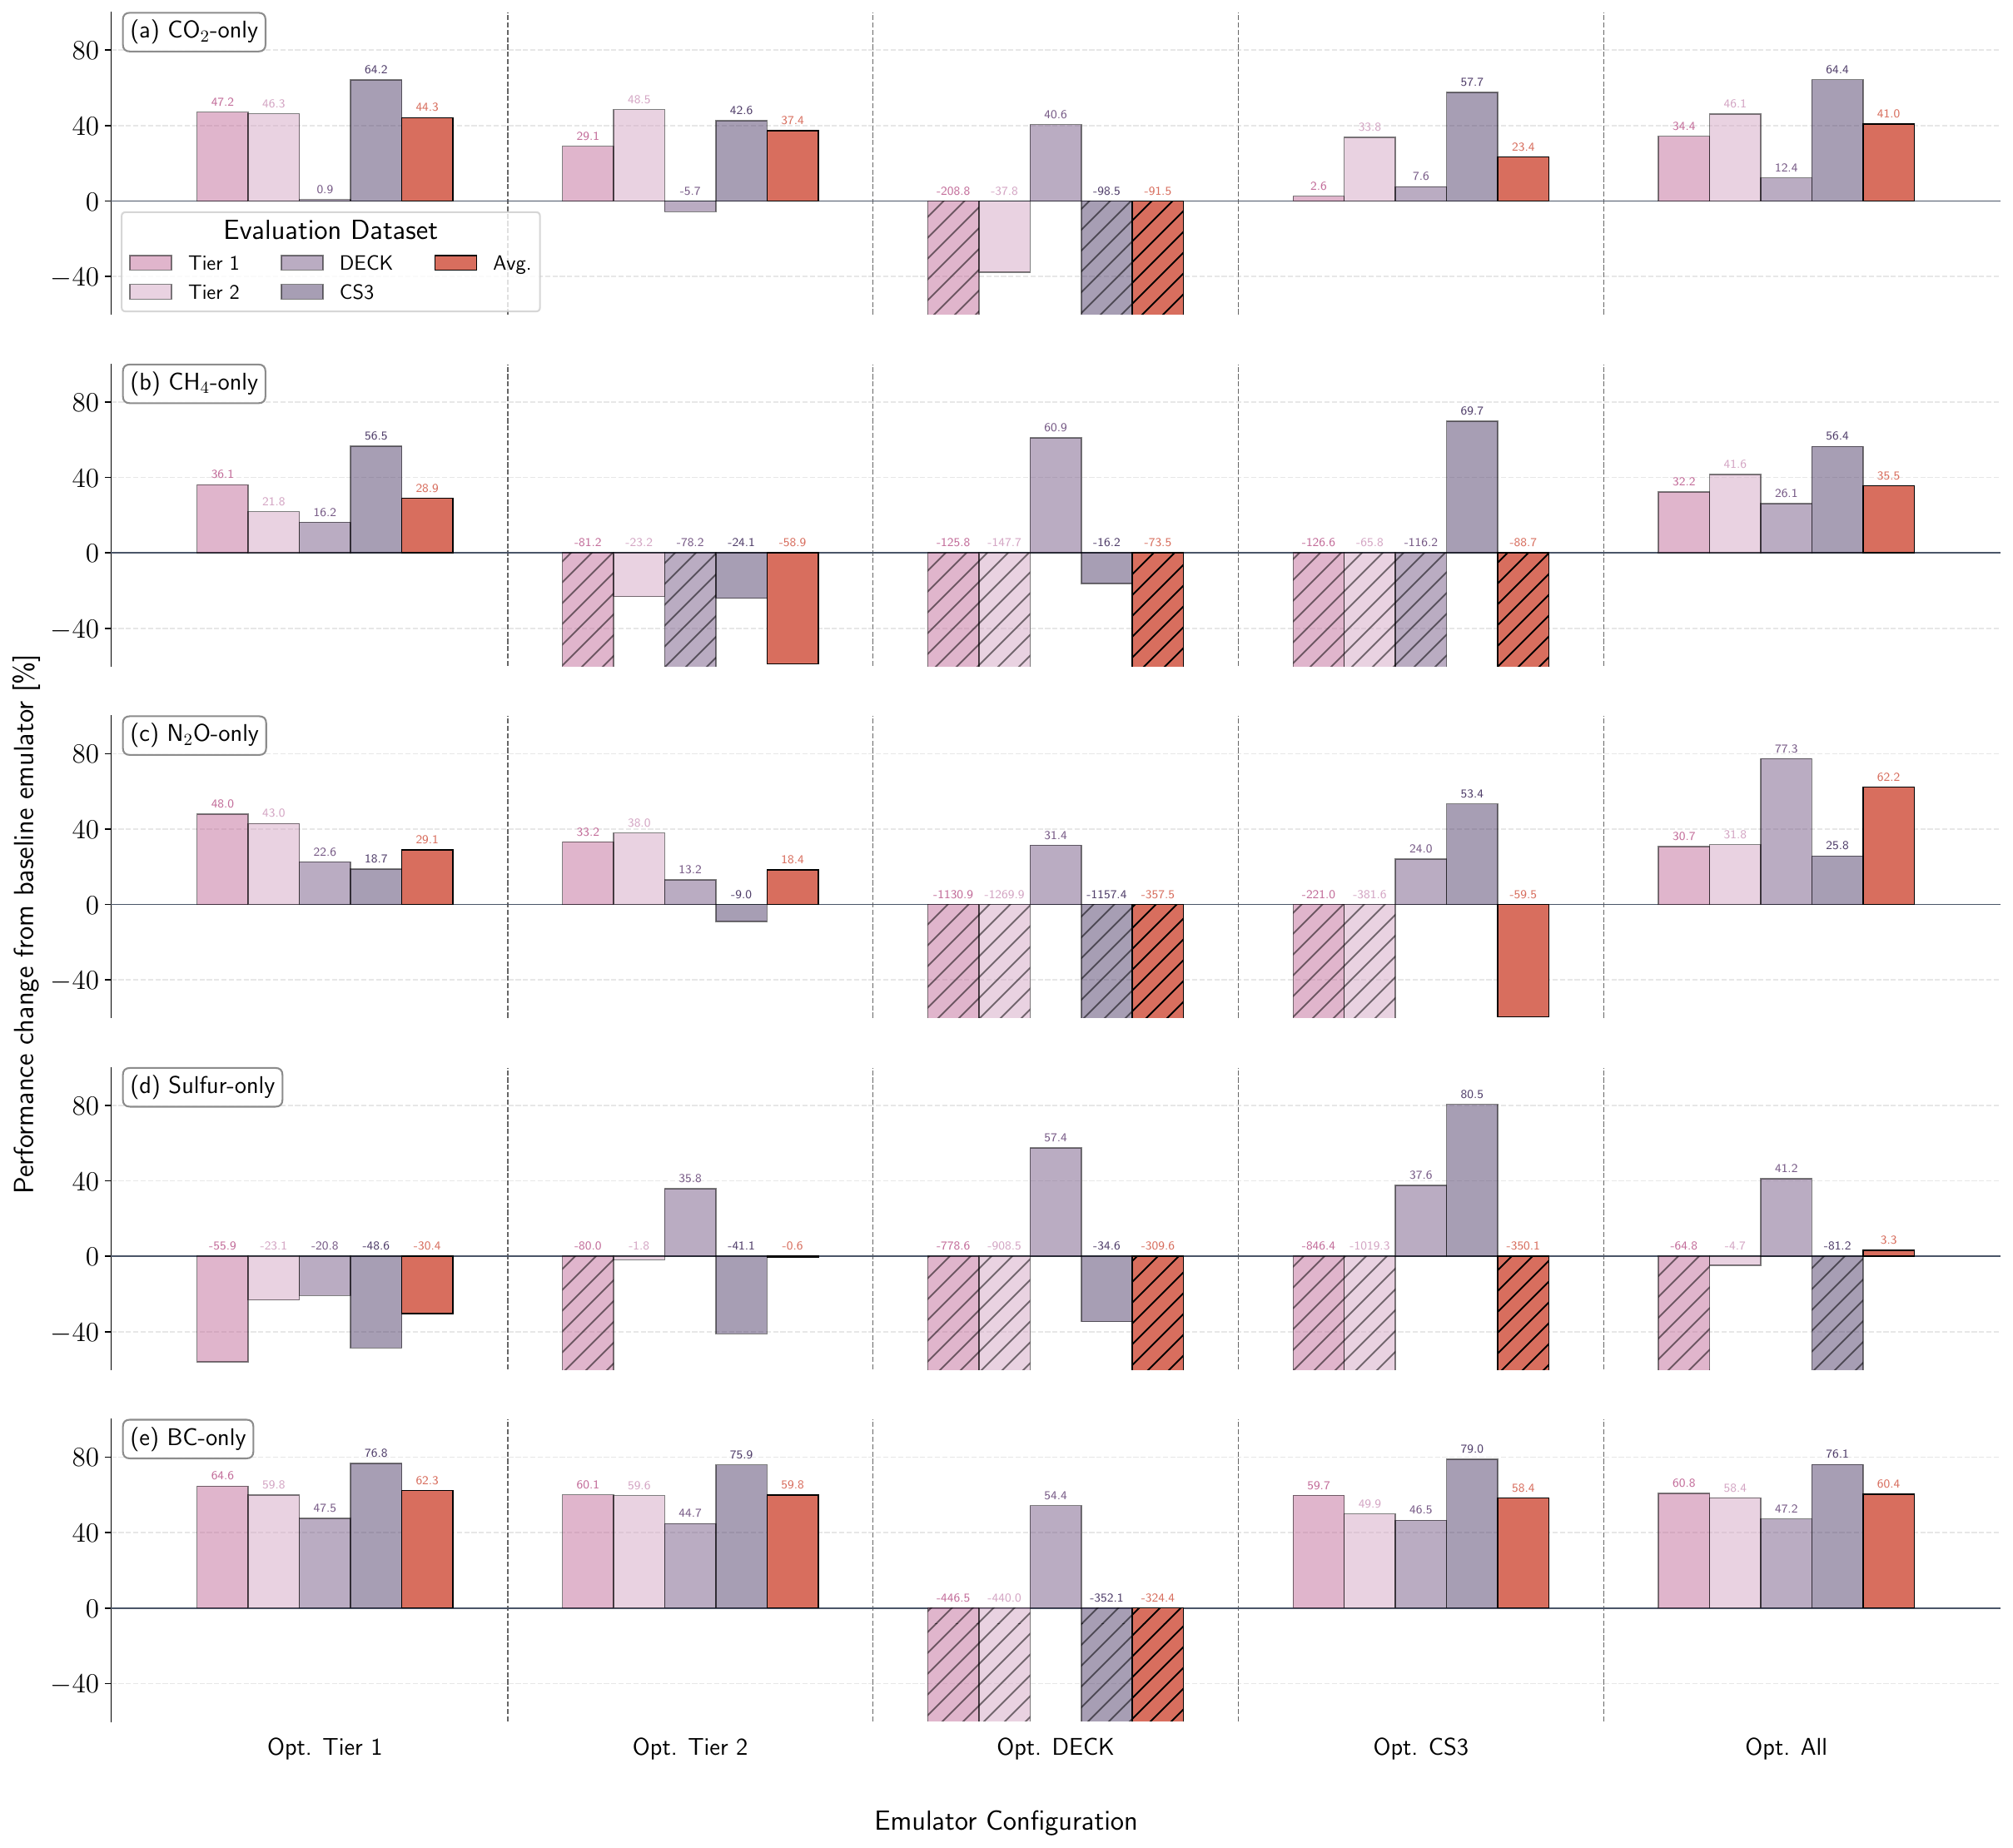}
    \caption{Relative change in emulator predictive skill (\gls{nrmse}) for optimized emulators compared to the baseline configuration. Panels show results for (a) CO$_2$-only; (b) CH$_4$-only; (c) N$_2$O-only; (d) Sulfur-only; (e) \gls{bc}. Positive values indicate reduced error (increased skill). Bars represent the average performance over all scenarios within a given evaluation dataset. Emulators are categorized by the subset of data used during optimization: ScenarioMIP Priority 1 and 2, DECK, CS3, and the full combined dataset. Hatching indicates a performance decrease that extends beyond the y-axis limits; y-axis limits are chosen for visual clarity.}
    \label{fig:SI_extended}
\end{figure}

\clearpage

\bibliographystyle{unsrtnat}
\bibliography{references}

\end{document}
